# Supplementary material for: Modeling observed gender imbalances in academic citation practices
Source: arXiv:2204.12555 source file (2022-04-26)
Supplement: Supplementary file 1 [file supp.pdf]

# Supplement: A model of gender imbalance in academic citation practices

Jennifer Stiso[1,2], Kendra Oudyk, Perry Zurn[3], and Dani S. Bassett[3,4,5,6,7,8]
[1]*Neuroscience Graduate Group, Perelman School of Medicine,*
*University of Pennsylvania, Philadelphia, PA 19104, USA*
[2]*Department of Bioengineering, School of Engineering and Applied Science,*
*University of Pennsylvania, Philadelphia, PA 19104, USA*
[3]*Department of Electrical & Systems Engineering, School of Engineering & Applied Science,*
*University of Pennsylvania, Philadelphia, PA 19104, USA*
[4]*Department of Neurology, Perelman School of Medicine,*
*University of Pennsylvania, Philadelphia, PA 19104, USA*
[5]*Department of Psychiatry, Perelman School of Medicine,*
*University of Pennsylvania, Philadelphia, PA 19104, USA*
[6]*Department of Physics & Astronomy, College of Arts & Sciences,*
*University of Pennsylvania, Philadelphia, PA 19104, USA*
[7]*The Santa Fe Institute, Santa Fe, NM 87501, USA and*
[8]*To whom correspondence should be addressed: dsb@seas.upenn.edu*

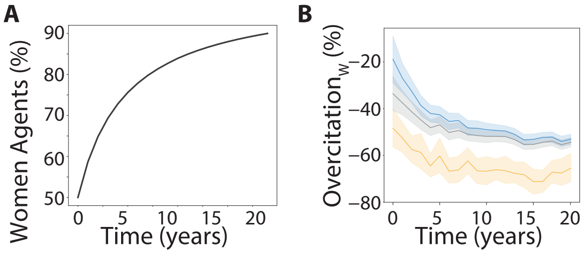


FIG. 1. **Replicating citation bias.** *(A)* The change in the proportion of women agents over time. *(B)* The overcitation of women over time for each agent gender, and the all agents - shown in grey (right).

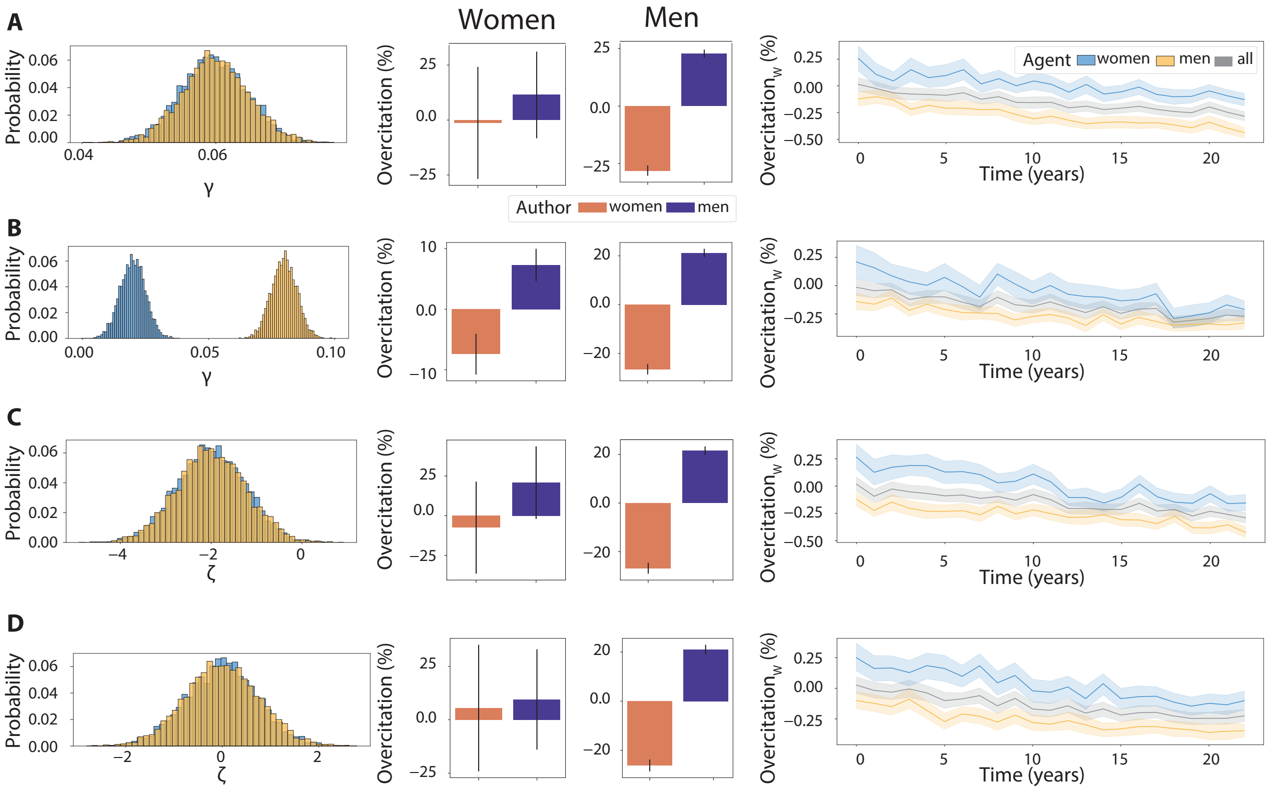


FIG. 2. **Replicating citation bias.** *(A)* Parameter distributions (left) total overcitation (middle) overcitation over time (right) when $\gamma$ is drawn for the same distribution for both genders. *(B)* Same as in panel *(A)*, but for a large difference in $\gamma$ values. *(C)* Same as in panel *(A)*, but with a $\zeta$ distribution centered on -2. *(D)* Same as in panel *(A)*, but with a $\zeta$ distribution centered on 0.

We asked if this pattern would reverse if the simulated agent population became woman dominated. We repeated our simulation with the proportion of women agents increasing from 50% to 90% over 20 years, rather than from 36% to 50%. We similarly find a decrease in the citation of women over time (linear model $overcitation_{w,w}\ time : \beta = -1.57 \times 10^{-2}, p = 8.61^{-7}$, $overcitation_{w,m} : \beta = -5.78 \times 10^{-3}, p = 3.38 \times 10^{-4}$). It is important to note that the new agents added to the population do not change the underlying network of authors available to chose citations from. Therefore, for agent proportions very far from the co-author bias (40%), only very large biases would be able to keep pace with the changing population.
